# Supplementary material for: On Tightness of Tsaknakis-Spirakis Descent Methods for Approximate Nash Equilibria
Source: arXiv:2107.01471 source file (2023-07-19)
Supplement: Supplementary file 1 [file Appendix_FullProof.tex]

\section{Full Proofs in the Main Body}\label{app:full-proof}
\subsection{Proof of Proposition~\protect{\ref{prop:construct-sp}}}

First, we show that $f_R(x^*,y^*)=f_C(x^*,y^*)$ is the necessary condition for $(x^*,y^*)$ to be a stationary point. We prove the contraposition. Suppose that $f_R(x^*,y^*)>f_C(x^*,y^*)$, then we have $f_R(x^*,y^*)>0$, which implies that $\max(Ry^*)>\T{x^*}Ry^*$. Therefore $\supp(x^*) \nsubseteq \suppmax(Ry^*)$.

Suppose without loss of generality that $1\in \suppmax(Ry^*)$, $2\notin\suppmax(Ry^*)$ and $2\in\supp(x^*)$. Let $E := \T{(1,-1,0,\cdots,0)}\in\R^m$. For sufficiently small $\theta_0>0$, we have $(x^*+\theta_0 E,y^*)\in \Delta_m\times\Delta_n$ and $f_R(x^*+\theta_0 E,y^*)>f_C(x^*+\theta_0 E,y^*)$. One can verify that
\begin{align*}
    Df(x^*,y^*,x^*+\theta_0 E,y^*)&=Df_R(x^*,y^*,x^*+\theta_0 E,y^*)\\
    &=-\theta_0 \T{E}Ry^*<0.
\end{align*}
Therefore $(x^*, y^*)$ is not a stationary point. The case of $f_C(x^*,y^*)>f_R(x^*,y^*)$ is similar.

Next, we prove that under the condition that $f_R(x^*,y^*)=f_C(x^*,y^*)$, $V(x^*,y^*)=f(x^*,y^*)$ if and only if (\ref{cond:sp-1}) and (\ref{cond:sp-2}) hold for some $\rho^*,w^*,z^*$.

Suppose $f(x^*,y^*)=V(x^*,y^*)$, by Proposition~\ref{prop:dual}, there exist $\rho^*,w^*,z^*$ such that
\[f(x^*,y^*) = \min_{x',y'} T(x^*,y^*,x',y',\rho^*,w^*,z^*).\]
Rewrite $T$ as
\begin{align*}
    T(x^*,y^*,x',y',\rho^*,w^*,z^*)&=\T{x'}A(\rho^*,y^*,z^*)+\T{B(\rho^*,x^*,w^*)}y' \\ 
    &+ \rho^* \T{x^*}Ry^* + (1 - \rho^*)\T{x^*}Cy^*.
\end{align*}
Notice that 
\begin{align*}
T(x^*,y^*,x^*,y^*,\rho^*,w^*,z^*) &=f(x^*,y^*)\\
&=\min_{x',y'} T(x^*,y^*,x',y',\rho^*,w^*,z^*).
\end{align*}
Therefore, 
\begin{align*}
    \supp(x^*) \subseteq \suppmin A(\rho^*,y^*,z^*), \\
    \supp(y^*) \subseteq \suppmin B(\rho^*,x^*,w^*)
\end{align*}
must hold.

Now suppose (\ref{cond:sp-1}) and (\ref{cond:sp-2}) hold. Similarly, we have
\begin{align*}
    V(x^*, y^*) &= \min_{x',y'} T(x^*,y^*,x',y',\rho^*,w^*,z^*) \\
    &= T(x^*,y^*,x^*,y^*,\rho^*,w^*,z^*) = f(x^*,y^*).
\end{align*}

\subsection{Proof of Lemma \protect{\ref{lemma:lambda*-mu*}}}

We have $\lambda^*,\mu^*\leq 1$ as all entries of $R$ and $C$ belong to $[0, 1]$. By the property of \SPn, $0\leq f(x^*,y^*)\leq T(x^*,y^*,x^*,z^*,\rho^*,w^*,z^*)=\rho^*\lambda^*$, therefore $\lambda^*\geq 0$. Similarly, $0\leq f(x^*,y^*)\leq T(x^*,y^*,w^*,y^*,\rho^*,w^*,z^*)=(1-\rho^*)\mu^*$, therefore $\mu^*\geq 0$.

\subsection{Proof of Lemma \protect{\ref{lemma:monotone-convex}}}

We only prove the first statement here and the second one is similar. Let $x_\alpha := \alpha w^*+(1-\alpha)x^*$, $y_\beta := \beta z^*+(1-\beta)y^*$.

Notice that 
\[F_C(\alpha,\beta) = \max(\T{C}x_\alpha) - \T{x_\alpha}Cy_\beta, \]
therefore is obviously convex and linear-piecewise in $\alpha$ with fixed $\beta$. A similar argument holds for $F_R(\alpha,\beta)$. We then show the increasing property for $F_R$. In fact, 
\[F_R(\alpha, \beta) = \max(Ry_\beta) - \T{x_\alpha}Ry_\beta, \]
therefore is linear in $\alpha$ with fixed $\beta$. Further by $\supp(w^*) \subseteq S_R(y^*)$ and Lemma~\ref{lemma:lambda*-mu*}, we have
\begin{align*}
    F_R(0, \beta) - F_R(1, \beta) &= (1 - \beta)\T{(w^* - x^*)}Ry^* + \beta\T{(w^* - x^*)}Rz^* \\
    &\geq \beta\lambda^* \geq 0,
\end{align*}
which shows that $F_R(\alpha, \beta)$ is decreasing with fixed $\beta$.

At last, to prove that $F_C(\alpha,\beta)$ is increasing in $\alpha$, by convexity, it suffices to show that $Df_C(x^*,y_\beta,w^*,y_\beta)\geq 0$. Note that $Df_R(x^*,y^*,w^*,y^*) \leq 0$. By the definition of \SPn, we must have
\begin{align}
    0&\leq Df(x^*,y^*,w^*,y^*)=Df_C(x^*,y^*,w^*,y^*)\notag\\
    &=\max_{S_C(x^*)}(\T{C}w^*)-\max(\T{C}x^*)+\T{(x^*-w^*)}Cy^*.\label{prove:Df1geq0}
\end{align}
Notice that $f_C(x^*,z^*)=0$ and $f_C(x,z^*)\geq 0$ for all valid $x$, so
\begin{align}
    0&\leq Df_C(x^*,z^*,w^*,z^*)\notag\\
    &=\max_{S_C(x^*)}(\T{C}w^*)-\max(\T{C}x^*)+\T{(x^*-w^*)}Cz^*.\label{prove:Df2geq0}
\end{align}
Combining (\ref{prove:Df1geq0}) and (\ref{prove:Df2geq0}), we have
\begin{align*}
    Df_C(x^*,y_\beta,w^*,y_\beta)&=\max_{S_C(x^*)}(\T{C}w^*)-\max(\T{C}x^*)+\T{(x^*-w^*)}Cy_\beta\\
    &=\beta Df_C(x^*,z^*,w^*,z^*)+(1-\beta)Df_C(x^*,y^*,w^*,z^*)\geq 0.
\end{align*}

\subsection{Proof of Lemma \protect{\ref{lemma:best-on-boundary}}}

Let $x_\alpha:=\alpha w^*+(1-\alpha)x^*$, $y_\beta:=\beta z^*+(1-\beta)y^*$. 
For the first part, by Proposition~\ref{prop:sp-equi}, $f_R(x^*,y^*)=f_C(x^*,y^*)=f(x^*,y^*)$. Meanwhile, Lemma~\ref{lemma:monotone-convex} shows that $f_C(x_\alpha,y^*)$ is an increasing function of $\alpha$, and $f_R(x_\alpha,y^*)$ is an decreasing function of $\alpha$, therefore $f(x_\alpha,y^*)=f_C(x_\alpha,y^*)\geq f_C(x^*,y^*)=f(x^*,y^*)$. Similarly, $f(x^*,y_\beta)=f_R(x^*,y_\beta)\geq f(x^*,y^*)$. As a result, $(x^*,y^*)$ is the minimum point of $f$ on $\Gamma_1$.

For the second part, suppose $f_C(w^*,z^*)\geq f_R(w^*,z^*)$. Again, by Lemma~\ref{lemma:monotone-convex} and a similar argument, $f(w^*,y_{\beta})=f_C(w^*,y_{\beta})\geq f_C(w^*,z^*)=f(w^*,z^*)\geq f(x_{\alpha^*},z^*)$. Therefore $\AdjSe=(x_{\alpha^*},z^*)$ is the minimum point on $\Gamma_2$. A similar argument holds for the case $f_R(w^*,z^*) > f_C(w^*,z^*)$.

\subsection{Proof of Lemma \protect{\ref{lemma:linearize}}}

We only prove the first statement, and the second one is similar. Let $y_\beta=\beta z^*+(1-\beta)y^*$. Since $F_C(\alpha,\beta)$ is a convex function of $\alpha$, it suffices to prove that $Df_C(w^*,y_\beta,x^*,y_\beta)=-Df_C(x^*,y_\beta,w^*,y_\beta)$ if and only if (\ref{cond:linearize1}) holds. One can verify that
\begin{align*}
    Df_C(w^*,y_\beta,x^*,y_\beta)&=\max_{S_C(w^*)}(\T{C}x^*)-\T{x^*}Ry_\beta-\max(\T{C}w^*)+\T{w^*}Cy_\beta,\\
    Df_C(x^*,y_\beta,w^*,y_\beta)&=\max_{S_C(x^*)}(\T{C}w^*)-\T{w^*}Ry_\beta-\max(\T{C}x^*)+\T{x^*}Cy_\beta.
\end{align*}
Sum up these two equations and we have
\begin{align*}
    &Df_C(w^*,y_\beta,x^*,y_\beta)+Df_C(x^*,y_\beta,w^*,y_\beta)\\
    =&\max_{S_C(x^*)}(\T{C}w^*)-\max(\T{C}w^*)+\max_{S_C(w^*)}(\T{C}x^*)-\max(\T{C}x^*)\leq 0.
\end{align*}
and the equality holds if and only if $S_C(x^*)\cap S_C(w^*)\neq\varnothing$.

\subsection{Proof of Proposition \protect{\ref{prop:stgy-comp}}}

$f\AdjFi\geq f\AdjSe$ and $f\AdjTh\geq f\AdjSe$ are directly deducted by Lemma~\ref{lemma:best-on-boundary}. We now prove the second part. 

If $f_R(w^*,z^*)=f_C(w^*,z^*)$, then by Lemma~\ref{lemma:monotone-convex} and Lemma~\ref{lemma:best-on-boundary}, we obtain that $\AdjSe=\AdjTh=(w^*,z^*)$.

Suppose now $f_C(w^*,z^*)>f_R(w^*,z^*)$. Let $x_\alpha:=\alpha w^*+(1-\alpha)x^*$, so $\AdjSe=(x_{\alpha^*},z^*)$. Notice that $f_R(x^*,z^*)\geq f_C(x^*,z^*)=0$, by intermediate value theorem and Lemma~\ref{lemma:monotone-convex}, the unique minimum point of $f$ on $\Gamma_2$, $\AdjSe$, lying on $\Phi=\{(x_\alpha,z^*):\alpha\in[0,1]\}$, is the intersection of $f_C$ and $f_R$. Again, by Lemma~\ref{lemma:monotone-convex}, $f_R$ is linear on $\Phi$ and $f_C$ is linear-piecewise on $\Phi$, therefore $\AdjSe$ coincides with $\AdjTh$ if and only if both $f_C$ is also linear on $\Phi$. By Lemma~\ref{lemma:linearize}, $f_C(x_\alpha,z^*)$ is linear on $\Phi$ if and only if $S_C(x^*)\cap S_C(w^*)\neq\varnothing$, which completes the proof of the case.

The case $f_R(w^*,z^*)>f_C(w^*,z^*)$ is symmetric, which we omit.

\subsection{Proof of Lemma \protect{\ref{lemma:ineq-for-est}}}

The value of $f\AdjTh$ is obtained immediately by definition. We now show the inequality holds. We only prove the case when $f_C(w^*,z^*)>f_R(w^*,z^*)$ and the other case is symmetric. Notice that 
\begin{align*}
    f\AdjTh &= \frac{f_R(x^*,z^*)(f_C(w^*,y^*)-\mu^*)}{f_C(w^*,y^*)+\lambda^*-\mu^*} \\
    &\leq \frac{(f_C(w^*,y^*)-\mu^*)}{f_C(w^*,y^*)+\lambda^*-\mu^*} \\
    &\leq \frac{1 - \mu^*}{1 + \lambda^* - \mu^*}.
\end{align*}
The second line holds as $f\AdjTh \geq 0$ and $f_R(x^*, z^*)\leq 1$, and the third line holds as
\[G(t) = \frac{t}{t + \lambda^*}\]
is increasing on $(0, 1 - \mu^*]$. Moreover, by the proof of Lemma~\ref{lemma:lambda*-mu*}, $\lambda^* > 0$ as $f(x^*, y^*) > 0$. As a result, the equality holds if and only if $f_C(w^*, y^*) = f_R(x^*, z^*) = 1$.

For the second part, notice that 
\[f(x^*, y^*) = \min_{x', y'}T(x^*, y^*, x', y', \rho^*, w^*, z^*).\]
Therefore,
\begin{align*}
    f(x^*,y^*)&\leq T(x^*,y^*,x^*,z^*, \rho^*,w^*,z^*)=\rho^*\lambda^*,\\
    f(x^*,y^*)&\leq T(x^*,y^*,w^*,y^*,\rho^*,w^*,z^*)=(1-\rho^*)\mu^*,
\end{align*}
which immediately derives that $f(x^*,y^*)\leq \min\{\rho^*\lambda^*,(1-\rho^*)\mu^*\}\leq\lambda^*\mu^*/(\lambda^*+\mu^*)$.

\subsection{Proof of Theorem \protect{\ref{thm:worst-case-exist}}}\label{app:thm:worst-case-exist}

We prove the theorem by verifying game (\ref{ex:tight-bound}) with stationary point $x^*=y^*=\T{(1,0,0)}$ and dual solution $\rho^*=\mu_0/(\lambda_0+\mu_0)$, $w^*=z^*=\T{(0,0,1)}$. Let $x_\alpha=\alpha w^*+(1-\alpha)x^*$, $y_\beta=\beta z^*+(1-\beta)y^*$.
\begin{enumerate}[label=\textit{Step \arabic*.}, fullwidth, listparindent=\parindent]
\item  Verify that $(x^*,y^*)$ is a \SPn. We have $f_R(x^*,y^*)=f_C(x^*,y^*)=b$. $A(\rho^*,y^*,z^*)=(-0.1\rho^*+(1-\rho^*)b)\T{e_3}$, therefore $\{1\}=\supp(x^*)\subset\{1,2,3\}=\suppmin(A(\rho^*,y^*,z^*))$. Condition (\ref{cond:sp-1}) holds. Similarly, condition (\ref{cond:sp-2}) holds, and the former statement is proved Proposition~\ref{prop:construct-sp}.
\item Verify that $S_C(x^*)\cap S_C(w^*)\neq\varnothing$ and $f_C(w^*,z^*)>f_R(w^*,z^*)$. The latter can be checked by direction calculation. One can calculate that $S_C(x^*)=\{2,3\}$ and $S_C(w^*)=\{2\}$, therefore their intersection is $\{2\}\neq\varnothing$. Consequently, by Proposition~\ref{prop:stgy-comp}, $f\AdjTh=f\AdjSe$ and by Lemma~\ref{lemma:linearize}, $f_C(x_\alpha,y_\beta)$ is a linear function of $\alpha$.
\item Verify that $\lambda^*=\lambda_0$, $\mu^*=\mu_0$, $f_R(x^*,z^*)=f_C(w^*,y^*)=1$, and $f(x^*,y^*)=b$. One can check these claims by calculation. Then by Lemma~\ref{lemma:est-for-stgy} and Lemma~\ref{lemma:ineq-for-est}, $f\AdjTh = f\AdjSe = b$.
\item Verify that $b\leq f(\alpha w^*+(1-\alpha)x^*,\beta z^*+(1-\beta)y^*)$ for any $\alpha,\beta\in[0,1]$.

First, we do a verification similar to step 2: $S_R(y^*)=\{2,3\}$ and $S_R(w^*)=\{2\}$, therefore $S_R(y^*)\cap S_R(z^*)=\{2\}\neq\varnothing$, and $f_R(x_\alpha,y_\beta)$ is a linear function of $\beta$.

Since $f_I(x_\alpha,y_\beta)\ (I\in\{R, C\})$ is a linear function of $\alpha$ or $\beta$, we can calculate the minimum point $(x^o(\beta),y_\beta)$ of $f$ given specific $\beta$.
\begin{align*}
    f_R(x_\alpha,y_\beta)&=b+(1-b)\beta-(b + (\lambda_0 - b)\beta)\alpha,\\
    f_C(x_\alpha,y_\beta)&=b - b\beta+(1 - b + (b - \mu_0)\beta)\alpha.
\end{align*}
and $x^o(\beta)$ satisfies
\begin{align*}
    &f_R(x^o(\beta),y_\beta)=f_C(x^o(\beta),y_\beta)\\
    \Longleftrightarrow\ & x^o(\beta)= \frac{\beta}{1+(\lambda_0-\mu_0)\beta}w^* + \left(1 - \frac{\beta}{1+(\lambda_0-\mu_0)\beta}\right)y^*.
\end{align*}

Now let
\[
    g(\beta):=f(x^o(\beta),y_\beta)=b + (1-b)\beta-\frac{(b + (\lambda_0 - b)\beta)\beta}{1+(\lambda_0-\mu_0)\beta}.
\]
As $\lambda_0 > \mu_0$, to prove that $\min_\beta g(\beta)=b$, it is sufficient to show
\begin{align*}
    (1-b)\beta(1+(\lambda_0-\mu_0)\beta)-(b + (\lambda_0 - b)\beta)\beta\geq 0.
\end{align*}
Or equivalently,
\begin{align*}
    h(\beta):=(1-2b)\beta+(b(1+\mu_0-\lambda_0)-\mu_0)\beta^2\geq 0.
\end{align*}

Notice that $h(\beta)$ has a negative coefficient on the square term, therefore $h(\beta)$ is a concave function. Further, we have $h(0)=0$ and $h(1)=1-2b+b(1+\mu_0-\lambda)-\mu_0>0$. By concavity, $h(\beta)\geq \beta h(1)+(1-\beta)h(0)\geq 0$.
\end{enumerate}

Now we complete the proof.

\subsection{Proof of Proposition \protect{\ref{prop:generator}}}\label{app:prop:generator}
To prove the first two statements, notice that by Proposition~\ref{prop:construct-sp}, Line~\ref{algline:SP1} and~\ref{algline:SP2} together form an equivalent condition such that $(x^*,y^*)$ is a \SP and $(\rho^*,w^*,z^*)$ is the corresponding dual solution.

Now we prove the latter two statements. By Lemma~\ref{lemma:best-on-boundary}, it suffices to prove that the algorithm outputs all games such that $f_C(w^*,z^*)>f_R(w^*,z^*)$, $f(x^*,y^*)\geq b$ and $f\AdjSe\geq b$. By Lemma~\ref{lemma:est-for-stgy} and \ref{lemma:ineq-for-est}, we already have 
\[\min\{f(x^*,y^*),f\AdjTh\}\leq b,\]
and the equality holds if and only if $f(x^*,y^*)=f\AdjTh=b$. By Proposition~\ref{prop:stgy-comp}, $f\AdjTh\geq f\AdjSe$, so it suffices to show $f(x^*,y^*)=f\AdjSe=f\AdjTh=b$ and $f_C(w^*,z^*)>f_R(w^*,z^*)$.

Line~\ref{algline:f-b} ensures that $f(x^*,y^*)=b$. Line~\ref{algline:br} and~\ref{algline:f1} together ensures that $f_R(x^*,z^*)=f_C(w^*,y^*)=1$. Line~\ref{algline:br} and~\ref{algline:lambda-mu} together ensures that $\lambda^*=\lambda_0$ and $\mu^*=\mu_0$. By Lemma~\ref{lemma:est-for-stgy} and~\ref{lemma:ineq-for-est}, these are equivalent conditions such that $f\AdjTh=b$, and it naturally leads to $f_C(w^*,z^*)>f_R(w^*,z^*)$ by Lemma~\ref{lemma:est-for-stgy}.

At last, by Proposition~\ref{prop:stgy-comp}, line~\ref{algline:2-3} is the equivalent condition such that $f\AdjTh=f\AdjSe$.
